# Supplementary material for: Impact Of Missing Data Imputation On The Fairness And Accuracy Of Graph Node Classifiers
Source: arXiv:2211.00783 source file (2022-11-01)
Supplement: Supplementary file 1 [file Appendix.tex]

\appendix
\section{Appendix}

\begin{figure}[ht!]
\centering
\includegraphics[scale = 0.8]{Figures/pdf/svd_val_1.pdf}
\caption{(a) Singular values, and (b) Cumulative energy contained in the first $d$ dimensions of $\Sigma$ (for Sweden dataset).}
\label{fig_svd_val_swe}
\end{figure}

\begin{figure}[ht!]
  \centering
  \includegraphics[width=\linewidth]{Figures/clust_goodness_swe.png}% picture filename
  \caption{Total hourly load of different clusters of consumers for one year in Sweden Dataset. The Figure is best seen in color.}
  \label{fig_clust_goodness_swe}
\end{figure}

\begin{figure}[ht!]
\centering
\includegraphics[scale = 0.6]{Figures/pdf/runtime_comparison.pdf}
\caption{Runtime of $k$-means algorithm ($k=80$) on load matrix without and with dimensionality reduction. Horizontal axis shows the increasing number of hours in the training set.}
\label{fig_clust_dim_time}
\end{figure}

\begin{figure*}[h!]
\centering
\begin{subfigure}{.25\textwidth}
  \centering
  \includegraphics[scale = 0.22] {Figures/swe_year_wise_tsne.png}
  \caption{Month wise labels}
  \label{fig_tsne_swe_month_wise}
\end{subfigure}%
\begin{subfigure}{.25\textwidth}
  \centering
  \includegraphics[scale = 0.22] {Figures/swe_weekend_wise_tsne.png}
  \caption{Weekdays/Weekends}
  \label{fig_tsne_swe_weekdays_weekends}
\end{subfigure}%
\begin{subfigure}{.25\textwidth}
  \centering
  \includegraphics[scale = 0.22] {Figures/swe_public_holiday_wise_tsne.png}
  \caption{Public Holiday}
  \label{fig_tsne_swe_public_holiday}
\end{subfigure}%
\begin{subfigure}{.25\textwidth}
  \centering
  \includegraphics[scale = 0.22] {Figures/swe_hours_of_day_wise_tsne.png}
  \caption{Hours of the Day}
  \label{fig_tsne_swe_hours}
\end{subfigure}
\caption{The t-SNE plots for different labels in case of Sweden Dataset.}
\label{fig_tsne_swe_labels}
\end{figure*}

\begin{figure*}[h!]
\centering
\begin{subfigure}{.25\textwidth}
  \centering
  \includegraphics[scale = 0.21] {Figures/ire_year_wise_tsne.png}
  \caption{Month wise labels}
  \label{fig_tsne_ire_month_wise}
\end{subfigure}%
\begin{subfigure}{.25\textwidth}
  \centering
  \includegraphics[scale = 0.21] {Figures/ire_weekend_wise_tsne.png}
  \caption{Weekdays/Weekends}
  \label{fig_tsne_ire_weekdays_weekends}
\end{subfigure}%
\begin{subfigure}{.25\textwidth}
  \centering
  \includegraphics[scale = 0.21] {Figures/ire_public_holiday_wise_tsne.png}
  \caption{Public Holiday}
  \label{fig_tsne_ire_public_holiday}
\end{subfigure}%
\begin{subfigure}{.25\textwidth}
  \centering
  \includegraphics[scale = 0.21] {Figures/ire_hours_of_day_wise_tsne.png}
  \caption{Hours of the Day}
  \label{fig_tsne_ire_hours}
\end{subfigure}
\caption{The t-SNE plots for different labels in case of Ireland Dataset.}
\label{fig_tsne_ire_labels}
\end{figure*}

\begin{figure}[h!]
\centering
\begin{subfigure}{.495\linewidth}
  \centering
    \includegraphics[width=\linewidth, page = 1] {Figures/correlation_plots.pdf}
    \caption{Australia dataset}
	\label{fig_corr_aus}%
\end{subfigure}%
\begin{subfigure}{.495\linewidth}
  \centering
   \includegraphics[width=\linewidth, page = 3] {Figures/correlation_plots.pdf}
    \caption{Sweden dataset}
	\label{fig_corr_swe}%
\end{subfigure}
\caption{Autocorrelation in the datasets. Sweden data has very low autocorrelation for all lag values (similarly Ireland data). The Australia data shows a slightly larger autocorrelation.}
\end{figure}

\begin{figure}[h!]
\centering
\begin{subfigure}{.33\linewidth}
  \centering
  \includegraphics[width=\linewidth]{Figures/pdf/hours_sum_a.pdf}
  \caption*{}
\end{subfigure}%
\begin{subfigure}{.33\linewidth}
  \centering
  \includegraphics[width=\linewidth]{Figures/pdf/hours_sum_b.pdf}
  \caption*{}
\end{subfigure}%
\begin{subfigure}{.33\linewidth}
  \centering
  \includegraphics[width=\linewidth]{Figures/pdf/hours_sum_3.pdf}
  \caption*{}
\end{subfigure}
\caption{\textsc{mape} of \textsc{fmf} for groups of households and longer durations. `Cluster: $i\,$' means households are grouped into $i$ clusters. Datasets: (a) Sweden (b) Ireland (c) Australia}
	\label{fig:mape_with_hour_agg}
\end{figure}

\subsection{Implementation Details}
A separate model is learned for each household in case of \textsc{arima} and \textsc{rf} while single model is learned for all households in case of \textsc{lstm} due to its computational complexity. Implementation details of these techniques are described as under.

\subsubsection{\textsc{arima}}
The input parameters for \textsc{arima} are the maximum and minimum number of autoregressive terms ($p$), the maximum and the minimum number of nonseasonal differences needed for stationarity ($q$), and the maximum and minimum number of lagged forecast errors ($d$). The output is an \textsc{arima} model fitted according to {\em Akaike Information Criterion}. We select $d = 0$, minimum $p = 1$, maximum $p = 5$, minimum $q = 1$, maximum $q = 5$. We fit Seasonal \textsc{arima}  (\textsc{sarima}), which is more suitable due to capturing seasonal information, \textsc{sarima}  $(p,q,d)(P,Q,D,S)$. The value of $S$ is $24$ because of seasonality effect. Maximum $P$ and maximum $Q$ values are taken as $2$, and maximum $D$ value is taken as $0$.
% \textcolor{red}{Expand it}
%\subsection{Arma}

\subsubsection{Random Forest (\textsc{rf})}
\textsc{rf} has been successfully used in \cite{kell2018segmenting} for \textsc{stlf} on clusters of household with accurate results motivating us to compare it with \textsc{fmf}. Two essential hyperparameters for \textsc{rf} are 'maximum attributes used in the individual tree' and the 'total number of trees', which are tuned using the validation set. 
As we increase the number of trees, the error starts decreasing, as shown in Figure \ref{random_forest_hyper_parameter}(b). Due to computational constraints, we select $100$ trees, and the maximum attributes used in each decision tree are $29$. This attributes count is chosen using the grid search on the validation set with mean squared error (\textsc{mse}) as error metric. In Figure \ref{random_forest_hyper_parameter} (a), \textsc{mse} has the least value against the attribute count of $29$. 
Since \textsc{rf} is invariant to scaling, we used Table \ref{hyper_parameters_description} features without scaling. A separate model is learned (with different hyperparameters) for each household in each dataset.  
% \textcolor{red}{Expand it}

% \begin{figure}[h!]
% 	\centering
% 	\footnotesize
% 	\begin{tikzpicture}
% 	\begin{axis}[title={},
% 	compat=newest,
% 	xlabel style={text width=5cm, align=center},
% 	%	xlabel style={align=center},
% 	xlabel={{\small (a) Number of Attributes for Individual Tree}},
% 	ylabel={MSE}, ylabel shift={-3pt},xtick={},
% 	height=0.53\columnwidth, width=0.53\columnwidth, grid=major,
% 	ymin=0.25, ymax=0.32,
% 	xtick={0,29,50,60,80,100},
% 	legend style={font=\tiny,draw=none,fill=none},
% 	legend entries={},
% 	]
% 	\addplot+[
% 	mark size=1pt,
% 	smooth,
% 	error bars/.cd,
% 	y fixed,
% 	y dir=both,
% 	y explicit
% 	] table [x={x}, y={y}, col sep=comma] {Data/mse_swe_RF_validation.csv};
% 	\end{axis}
% 	\end{tikzpicture}%
% 	\hspace{-1cm}
% 	\begin{tikzpicture}
% 	\begin{axis}[title={},
% 	compat=newest,
% 	xlabel style={text width=3.5cm,align=center},
% 	xlabel style={align=center},
% 	xlabel={{\small (b) Total Number of \\ Trees}},
% 	ylabel shift={-3pt},xtick={},
% 	height=0.53\columnwidth, width=0.53\columnwidth, grid=major,
% 	ymin=0.22, ymax=0.42,
% 	legend style={font=\tiny,at={(1,0.7)},anchor=south east,legend style={draw=none},legend style={fill=none}},
% 	legend entries={},
% 	]
% 	\addplot+[
% 	mark size=1pt,
% 	smooth,
% 	error bars/.cd,
% 	y fixed,
% 	y dir=both,
% 	y explicit
% 	] table [x={x}, y={y}, col sep=comma] {Data/mse_swe_RF_validation_num_of_trees.csv};
% 	\end{axis}

% 	\end{tikzpicture}%
% 	\caption{Hyperparameter tuning of Random Forest for a single Household of Sweden dataset.}
% 	\label{random_forest_hyper_parameter}
% \end{figure}

\begin{figure}[h!]
\centering
\begin{subfigure}{.25\textwidth}
  \centering
  \includegraphics[scale = 0.8]{Figures/pdf/num_of_attr.pdf}
  \caption*{}
\end{subfigure}%
\begin{subfigure}{.25\textwidth}
  \centering
  \includegraphics[scale = 0.8]{Figures/pdf/num_of_trees.pdf}
  \caption*{}
\end{subfigure}%
\caption{Hyperparameter tuning of Random Forest for a single Household of Sweden dataset.}
	\label{random_forest_hyper_parameter}
\end{figure}

\subsubsection{\textsc{lstm}}
The architecture of \textsc{lstm} scheme proposed in \cite{kong2019short} consists of $2$ hidden layers with $20$ nodes in each layer. A simple neural network with sigmoid activation function is used to ensemble the final prediction. The features used in \textsc{lstm} are shown in Table \ref{hyper_parameters_description}. The number of previous time stamps used in the forecasting is $6$.
Furthermore, \textsc{mse} with Adam optimizer \cite{kingma2014adam} is used to perform training for $100$ epochs. Since \textsc{lstm} contains a large number of weights, learning these weights requires huge data. We test separate \textsc{lstm} models on individual households and a single model on all households. Due to less amount of data, a separate model on individual households performs poorly as compared to a single model on all households. Therefore, we only include the results of a single model for all households on each dataset. 

%\subsubsection{Multiple linear regression}
%For this algorithm, we directly use the results given in \cite{lusis2017short} for comparison with \textsc{fmf}.
%
%\subsubsection{Regression trees}
%Same as MLR, we use the results given in \cite{lusis2017short} for the comparison purpose rather than implementing this algorithm.
%
%\subsubsection{Support Vector Regression}
%To compare \textsc{fmf} with SVR, we use the reported results in \cite{lusis2017short}.
%
%\subsubsection{Neural Network}
%We did not implement the NN approach. We use the results reported in \cite{lusis2017short} to compare \textsc{fmf} with the NN. To make further comparisons with another state-of-the-art approach, we use the results of NN given in \cite{kell2018segmenting} and compare them with the computed results using \textsc{fmf}.
%
%\subsubsection{Support Vector Regression}
%Rather than implementing SVR, we use the results reported in \cite{kell2018segmenting} for the comparison purpose.

\begin{table}[h!]
	\centering
	\begin{tabular}{llp{4.8cm}}
		\hline
		Index &\multicolumn{1}{c}{Variable} & \multicolumn{1}{c}{Description}  \\ [0.5ex] 
		\hline\hline
		1-24 & Hours & One hot encoding vector\\
		25-31 & Day of Week & One hot encoding vector \\
		32-62 & Day of Month & One hot encoding vector\\
		63-74 & Month & One hot encoding vector\\
		75-85 & Lagged Input & 3 previous hours of same day, 4 hours of previous day including hour to be predicted, 4 hours of same day of previous week including hour to be predicted\\
		86 & Public Holiday & Boolean input\\
		87 & Temperature & Single numeric input\\
		88 & Wind Speed & Single numeric input \\
		89 & Humidity & Single numeric input\\
		[1ex] 
		\hline
	\end{tabular}
	\caption{Input parameters for the classification algorithms.}
	\label{hyper_parameters_description}
\end{table}
